# Supplementary material for: Dichography: Two-frame Ultrafast Imaging from a Single Diffraction Pattern
Source: arXiv:2508.20153 ancillary file (2026-02-27)
Supplement: Supplementary file 1 [file supplementary.pdf]

# Dichography: Two-frame Ultrafast Imaging from a Single Diffraction Pattern

## Supplemental Material

### S1 Brightness requirements of Dichography

#### S1.1 Simulation of realistic diffraction data

Similar to conventional CDI, the brightness of the diffraction image has a strong impact on the capability of *Dichography* to separate and retrieve the two frames contributing to the scattering. In this section, we empirically investigate this aspect by analyzing the performance of the method on simulated data.

Simulated diffraction images are produced following the procedure illustrated in Fig. S1. The inner part of the data is removed to mimic the presence of a hole in the detector, as required in real experiments to prevent damage from the transmitted FEL beam. The diameter of the missing central region is set to 10 % of the linear matrix size.

Statistical noise from photon counting is also added to the data. This noise depends on the overall signal brightness, i.e., the total photon count. The simulated noisy data,  $I^m$ , is generated using the following expression:

$$I_{ij}^m = \mathcal{P} \left[ \frac{I_{ij}^A}{\sum I_{ij}^A} \cdot N_{\text{ph}}^A \right] + \mathcal{P} \left[ \frac{I_{ij}^B}{\sum I_{ij}^B} \cdot N_{\text{ph}}^B \right] \quad (\text{S1})$$

where  $\mathcal{P}[x]$  denotes a Poisson-distributed random integer with mean  $x$ , and  $I^A$  and  $I^B$  are the simulated scattering intensities from  $\rho^A$  and  $\rho^B$ , respectively. The parameters  $N_{\text{ph}}^A$  and  $N_{\text{ph}}^B$  specify the desired total number of scattered photons for each contribution.

In this way, the simulated data  $I_{ij}^m$  represents photon counts for each pixel  $(i, j)$ , with a total photon yield  $\sum I_{ij}^m$  approximately equal to  $N_{\text{ph}}^A + N_{\text{ph}}^B$ , subject to statistical fluctuations.

For testing purposes, it is convenient to re-write the total photon counts of the two signals,  $N_{\text{ph}}^A$  and  $N_{\text{ph}}^B$ , as follows:

$$\begin{aligned} N_{\text{ph}}^A &= N_{\text{ph}}^{\text{tot}} \cdot \alpha \\ N_{\text{ph}}^B &= N_{\text{ph}}^{\text{tot}} \cdot (1 - \alpha) \end{aligned} \quad (\text{S2})$$

Here,  $N_{\text{ph}}^{\text{tot}}$  indicates the total number of recorded photons after summing the two contributions, while  $\alpha \in (0, 1)$  defines the balance between them. For example,  $\alpha = 0.5$  means the contributions are perfectly balanced — so if  $N_{\text{ph}}^{\text{tot}} = 2 \cdot 10^6$ , then  $N_{\text{ph}}^A = N_{\text{ph}}^B = 1 \cdot 10^6$ . A value of  $\alpha = 0.8$  instead means that 80 % of the scattered photons originate from  $\rho^A$  (i.e.,  $N_{\text{ph}}^A = 1.6 \cdot 10^6$ ) and 20 % from  $\rho^B$  (i.e.,  $N_{\text{ph}}^B = 4 \cdot 10^5$ ).

In the following sections, the reconstruction capabilities of *Dichography* are tested for different total signal brightness values  $N_{\text{ph}}^{\text{tot}}$  and varying balance  $\alpha$  between the two scattering contributions. In those tests, the support function is supposed to be unknown, and it is retrieved in the reconstruction process.

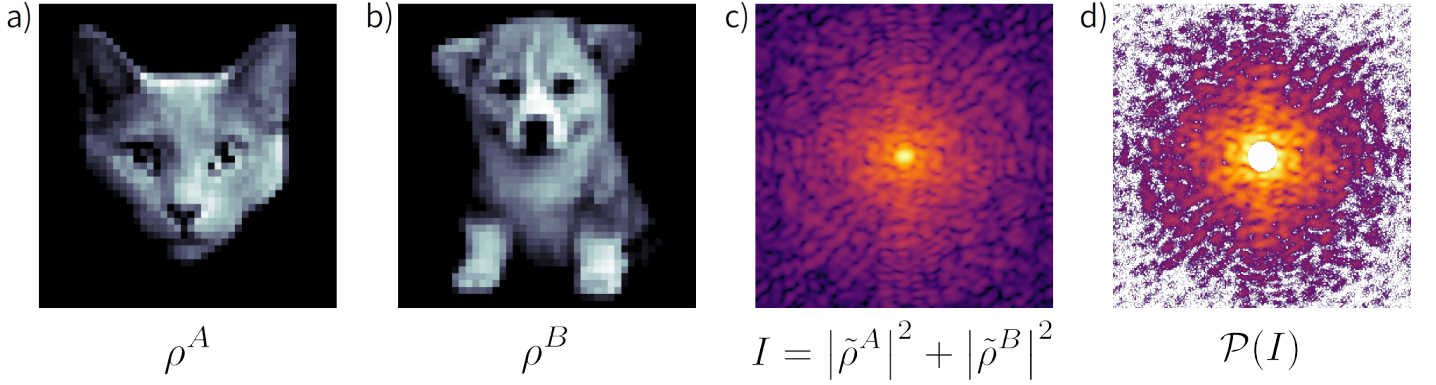

Figure S1: Example of simulated data. The simulations are performed by filling two real-valued matrices of size  $266 \times 256$  pixels with two different images, as shown in a) and b). The scattered field is calculated as the incoherent sum of the two contributions, shown in c). Realistic data, shown in d), is produced by adding photon noise and removing the central part of the pattern, which is typically missing in FEL experiments to avoid detector damage from the transmitted beam.

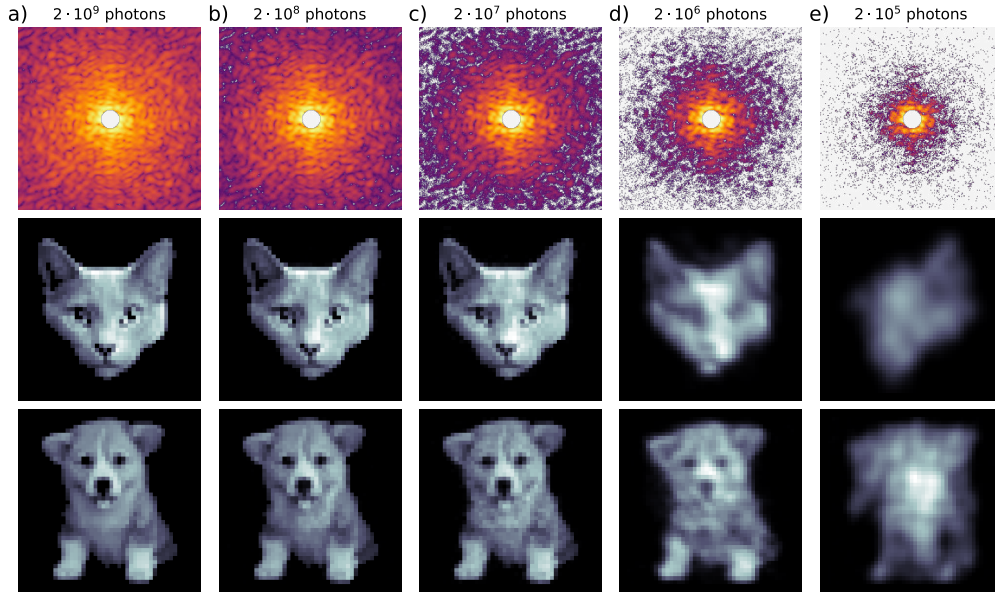

Figure S2: Impact of brightness on the reconstruction. Each subfigure a) to e) contains the diffraction image and the two reconstructed frames for different photon yields in the data.

## S1.2 Effects of overall brightness

In this section, the results are tested for different values of the total photon count  $N_{\text{ph}}^{\text{tot}}$ , while keeping the individual contributions balanced at 50 % ( $\alpha = 0.5$ ). Tests are performed on two different samples, and the corresponding results are presented in Fig. S2 and Fig. S3.

The data in Fig. S2 originate from two densities whose spatial extensions (i.e., support functions) do not fully overlap and have significantly different shapes. In this case, the two frames are accurately retrieved down to  $2 \cdot 10^7$  photons (Fig. S2c). Separation is still possible at  $2 \cdot 10^6$  photons, although with a noticeable loss in spatial resolution (Fig. S2d). The reconstruction fails entirely at a photon yield of  $2 \cdot 10^5$ .

The problem becomes more brightness-sensitive in cases where the two samples have similar shapes, and the support function of one frame can fully contain the other. This situation is investigated in Fig. S3, and it is conceptually similar to the two-color case, where the sample is imaged with two different photon energies. The

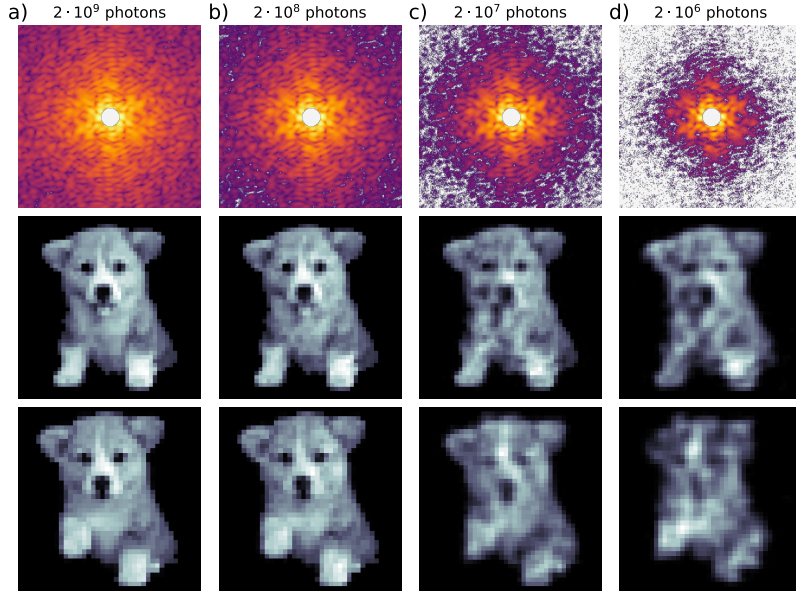

Figure S3: Impact of brightness on the reconstruction. Each subfigure a) to d) contains the diffraction image and the two reconstructed frames for different photon yields in the data.

data for this example are produced by taking two similar images (the dog's mouth is open in the first frame, the paw is raised in the second) and scaling one to a size that differs by 10 % in pixel count. This mimics scattering from two photon energies with a 10 % difference in wavelength, making the second frame (corresponding to the longer wavelength) smaller in spatial extension.

Fig. S3 reveals a different behavior compared to Fig. S2. On the one hand, the ability to distinguish the two overall shapes persists down to  $2 \cdot 10^6$  photons (Fig. S3d). On the other hand, *Dichography* struggles more to resolve fine details, with reconstruction artifacts already dominating at  $2 \cdot 10^7$  photons (Fig. S3c).

### S1.3 Relative intensities of the two frames

The second aspect investigated here concerns the relative intensity between the two frames, tuned via the parameter  $\alpha$  in Eq. (S2).

Values of  $\alpha = 0.5, 0.7, 0.8, 0.9$ , and  $0.95$  are probed, corresponding to 50 %-50 %, 70 %-30 %, 80 %-20 %, 90 %-10 %, and 95 %-5 % photon distributions between  $\rho^A$  and  $\rho^B$ .

The first test, shown in Fig. S4, is performed on data with high brightness, with a total photon count of  $N_{\text{ph}}^{\text{tot}} = 2 \cdot 10^9$ . In the figure, the reconstruction of the second frame (dog) is shown twice: once normalized on an independent color scale, and once using the same scale as the first frame. This highlights differences in scattering intensity and the resulting density contrast. In this high-brightness case, all reconstructions were successful, even for the highly unbalanced case in Fig. S4e, where the brightness of the first frame is 19 times higher.

The same photon balance configurations are tested at decreasing total photon counts:  $N_{\text{ph}}^{\text{tot}} = 2 \cdot 10^8$ ,  $2 \cdot 10^7$ , and  $2 \cdot 10^6$ , shown in Fig. S5, Fig. S6, and Fig. S7, respectively.

From comparing these figures, it can be deduced that decreasing photon yield not only impacts reconstruction quality (as discussed in Fig. S2 and Fig. S3), but also makes *Dichography* increasingly sensitive to unbalanced contributions between the two signals. This effect can be explained and understood through statistical considerations of shot noise.

The primary source of noise in the data arises from the statistical nature of photon detection. As described in Eq. (S1), photon statistics follow a Poisson distribution. This implies that for a scattering signal with an

expected value  $I_{ij}$  (expressed in photon counts), the standard deviation — i.e., the statistical fluctuation — is  $\sqrt{I_{ij}}$ .

Since the recorded signal is the sum of two independent Poisson-distributed random variables, the total measured intensity has an expected value of  $I_{ij}^A + I_{ij}^B$  and a standard deviation of  $\sqrt{I_{ij}^A + I_{ij}^B}$ . Assuming that the first frame of the reconstruction is perfectly retrieved, i.e.,  $I_{ij}^A$  is known exactly, the remaining signal attributed to the second frame can be defined as:

$$I_{ij}^{B_m} = \mathcal{P} [I_{ij}^A + I_{ij}^B] - I_{ij}^A \quad (\text{S3})$$

with statistical properties:

$$\begin{aligned} \mu_{ij}^{B_m} &= I_{ij}^B = (1 - \alpha) \cdot I_{ij} \\ \sigma_{ij}^{B_m} &= \sqrt{I_{ij}^A + I_{ij}^B} = \sqrt{I_{ij}} \end{aligned} \quad (\text{S4})$$

The ability to extract meaningful information from  $I_{ij}^{B_m}$  depends on achieving a sufficient Signal-to-Noise Ratio (SNR). To resolve the signal reliably, the SNR must exceed a minimum threshold  $\mathcal{S}$ :

$$\text{SNR}_{ij}^{B_m} = \frac{\mu_{ij}^{B_m}}{\sigma_{ij}^{B_m}} = (1 - \alpha) \cdot \sqrt{I_{ij}} > \mathcal{S} \quad (\text{S5})$$

This leads to a condition on the balance parameter  $\alpha$ :

$$\alpha < 1 - \frac{\mathcal{S}}{\sqrt{I_{ij}}} \quad (\text{S6})$$

The condition presented in Eq. (S6) is thus a simplified view of the system and cannot be interpreted in a fully quantitative manner. Still, it captures the qualitative behavior observed in Figures S4, S5, S6, and S7. Specifically, given a minimum SNR value  $\mathcal{S}$  necessary for successful reconstruction, the higher the brightness of the pattern  $I_{ij} \propto N_{\text{ph}}^{\text{tot}}$ , the closer  $\alpha$  can be to 1 (i.e., a strong imbalance between the signals), as shown in Fig. S4. Conversely, the lower the overall pattern intensity, the smaller the allowed values of  $\alpha$ , as illustrated, for example, in Fig. S7.

The considerations made so far concern specific pixel coordinates, and low SNR values may have different impact on a CDI reconstruction. For example, if low SNR values are at high momentum transfer (close to the edges of the detector), the reconstruction outcome is typically successful and only the spatial resolution is affected. When low SNR values are already appearing at low momentum transfer, close to the center of the detector, the CDI reconstruction typically completely fails. Furthermore, the amount of noise to which the reconstruction is tolerant is dependent on the sample, and in particular its size: higher *oversampling degrees* (i.e. smaller samples) are typically much more resilient to noise than more extended samples, due to the higher information redundancy in the scattering image and lower number of unknowns to retrieve.

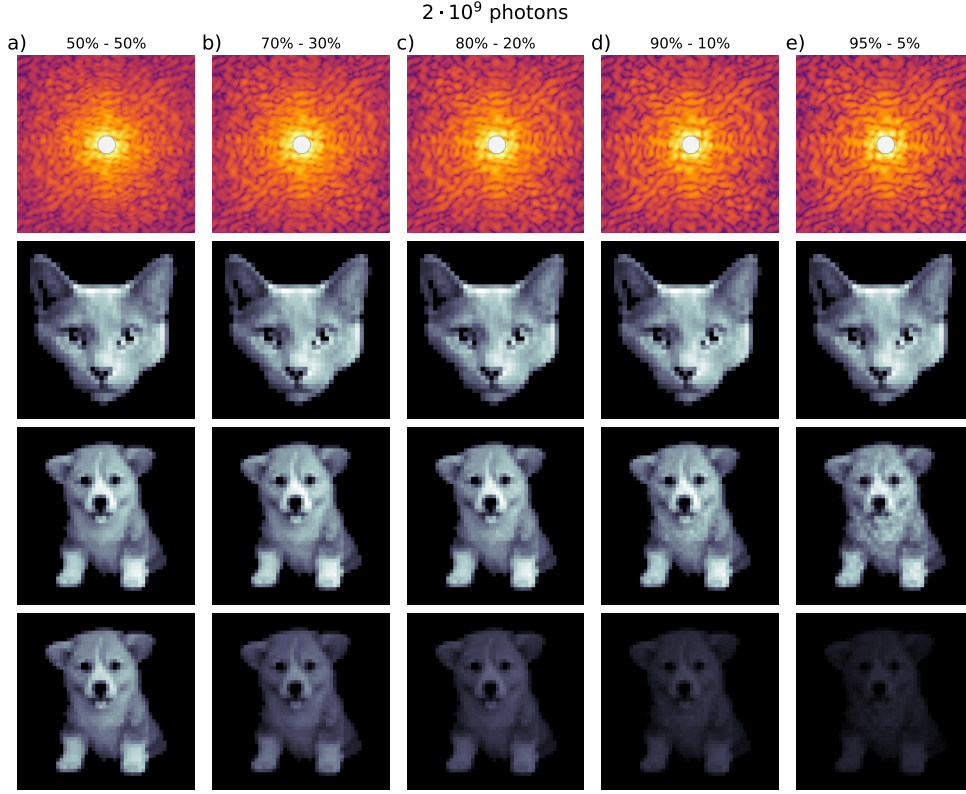

Figure S4: Impact of different relative brightness on the reconstruction for a total photon count of  $2 \cdot 10^9$ . Each subfigure a) to e) contains the diffraction image and the two reconstructed frames for different photon yields in the data. The second frame of the reconstruction is reported twice, in the third row with renormalized brightness, while in the fourth with the same color scale of the first frame.

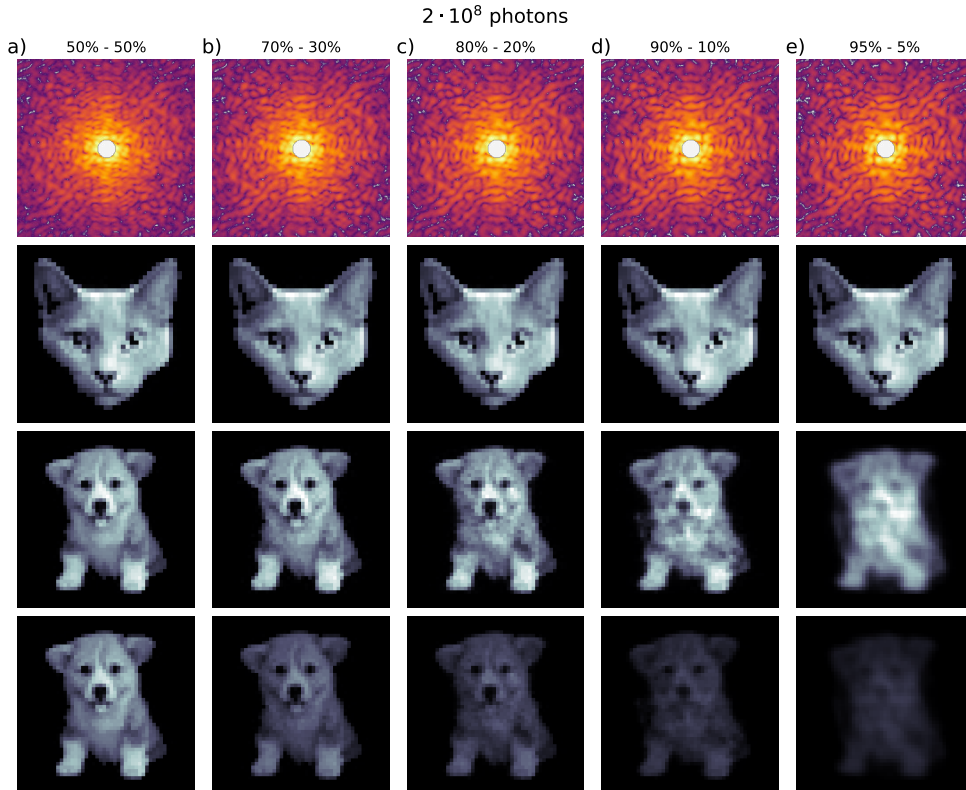

Figure S5: Impact of different relative brightness on the reconstruction for a total photon count of  $2 \cdot 10^8$ . The figure is organized as Fig. S4.

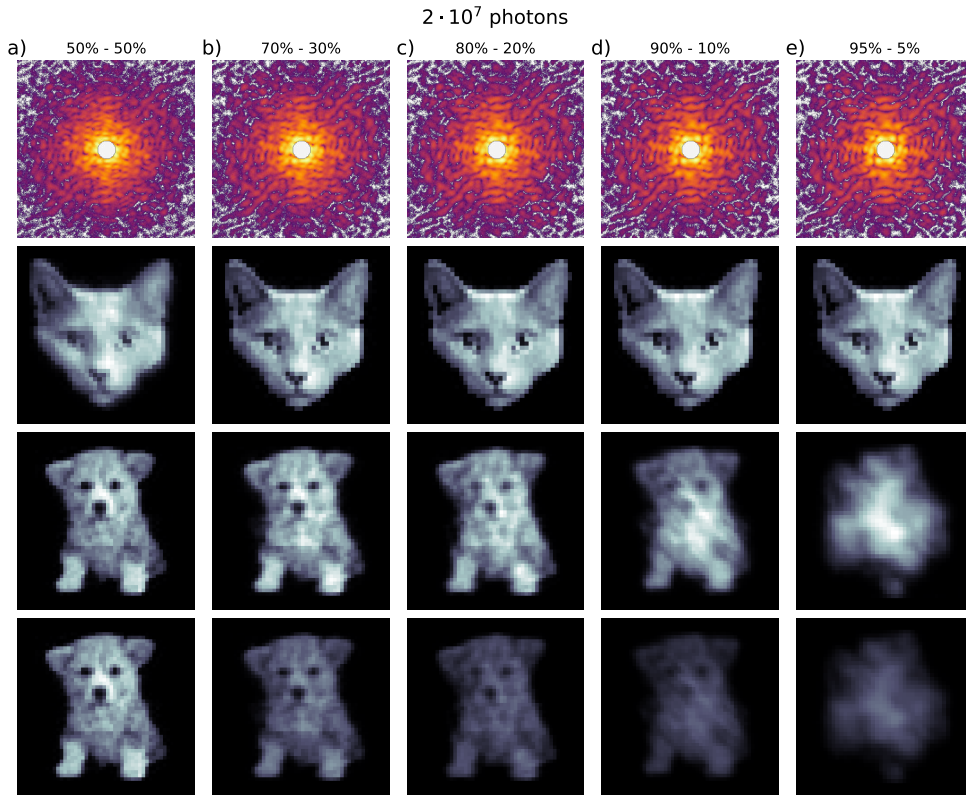

Figure S6: Impact of different relative brightness on the reconstruction for a total photon count of  $2 \cdot 10^7$ . The figure is organized as Fig. S4.

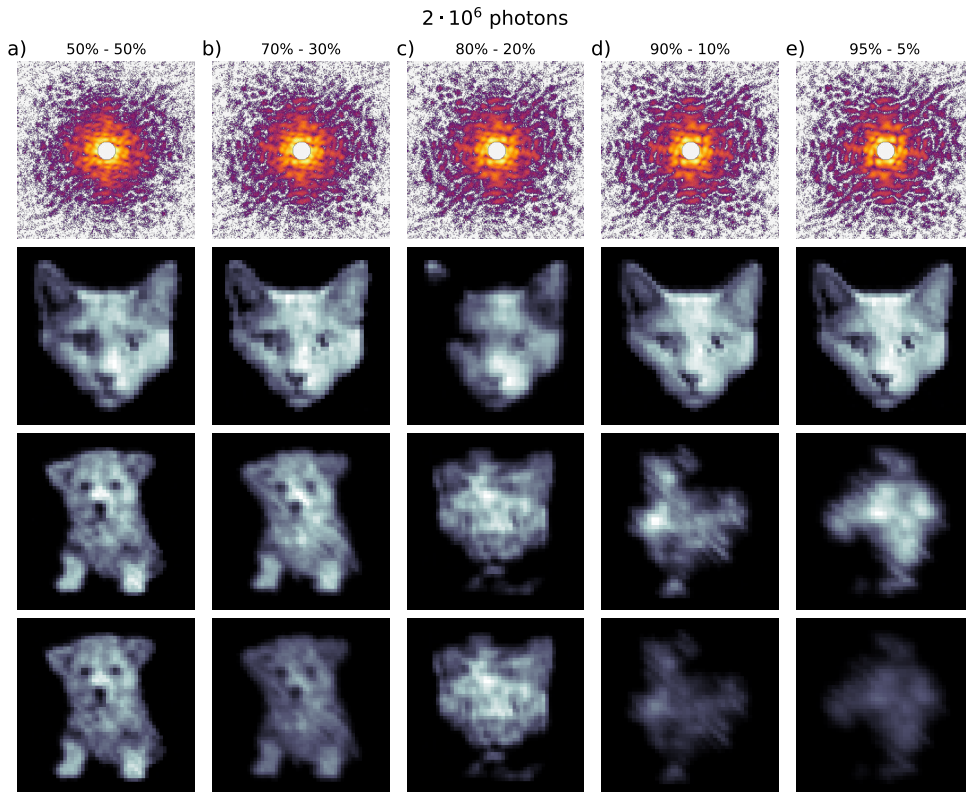

Figure S7: Impact of different relative brightness on the reconstruction for a total photon count of  $2 \cdot 10^6$ . The figure is organized as Fig. S4.

## S1.4 Intensity dependence for Droplet-CDI

As discussed in Sec. III B of the main manuscript, the two-color operational mode of the XFEL comes with a reduction in the overall intensity of the two pulses, compared to the single-color mode. This feature is significantly impacting imaging experiments, which are inherently *photon-hungry*. Two-color patterns from xenon-doped superfluid helium nanodroplets allow dichrographic imaging only under optimal conditions for both FEL pulses using the Droplet-CDI approach [1]. In this section, we perform a systematic analysis on the performance of *Dichography* on simulated data, by tuning the overall brightness to better understand and evaluate the results presented in Sec. III B.

Simulations are performed for a superfluid helium nanodroplet with a diameter of 420 nm. Inside the droplet, a structure resembling a filament of xenon aligned along a quantum vortex [2, 3] is added. The filament thickness is set to 5 nm. The density of the materials is tuned to  $0.125 \text{ g/cm}^3$  for superfluid helium and  $3.000 \text{ g/cm}^3$  for xenon. The scattering cross sections of the two components have been adjusted accordingly.

Like the tests presented in Sec. S1.2, the performance of *Dichography* is probed for different numbers of total scattered photons  $N_{\text{ph}}^{\text{tot}}$ . The relative brightness between the two frames is adjusted to match the one measured for the experimental pattern presented in Fig. 4a of the main manuscript, where the signal from the 1.2 keV *probe* pulse scatters 64 % more photons than the 1.0 keV *pump* pulse. This is achieved by setting the photon balance parameter  $\alpha$  to 0.38 (see Eq. (S2)). The structure of the xenon filament has been slightly modified between the two frames, to highlight whether the information is correctly separated.

The simulated patterns and the corresponding *Dichography* reconstructions are shown in Fig. S8a-g, for different total intensities. The intensity, indicated in terms of total scattered photons, can be quantitatively compared with the experimental data. In fact, from the experimental reconstructions in Fig. 4, the corresponding total yield of diffracted photons can be estimated to be  $N_{\text{ph}}^{\text{tot}} = 2.3 \cdot 10^6$  for Fig. 4a and  $N_{\text{ph}}^{\text{tot}} = 1.5 \cdot 10^6$  for Fig. 4d.

The first row (Fig. S8a) corresponds to a total photon yield, indicated at the right end, about 25 times higher than that observed in the experiment. The higher intensity can also be qualitatively deduced by visual comparison of the scattering image with those reported in Fig. 4a and 4d. At such a high photon count, the corresponding two reconstructed frames show very high quality, with sharp density profiles that also clearly highlight the high achieved resolution. The structural difference between the two frames is well identifiable, with the right end of the filament being more stretched and straighter in the 1.2 keV frame.

With the reduction in intensity down to  $5 \cdot 10^6$  photons, in Fig. S8b and S8c, the structural properties of the two frames remain consistent. The lower number of photons affects mostly the outer area of the detector, reducing the actual resolution of the reconstructions. Due to this loss in resolution, the reconstructed xenon structure appears thicker with decreasing brightness.

The range of photon counts between  $3 \cdot 10^6$  and  $1.5 \cdot 10^6$ , in Fig. S8d-f, corresponds to a transition region between reliable reconstruction conditions and situations that lead to reconstruction failure. This is also the range in which the experimental reconstructions shown in Fig. 4 lie, with  $N_{\text{ph}}^{\text{tot}} = 2.3 \cdot 10^6$  and  $N_{\text{ph}}^{\text{tot}} = 1.5 \cdot 10^6$ , respectively.

These simulations give insight into how a reconstruction fails with reduced brightness. The first signs are fluctuations in the density signal along the filaments, with regions of higher or lower scattering cross section (Fig. S8d). Here, the filaments still retain their correct structure. At even lower photon yields (Fig. S8e), structural artifacts start to appear on top of the density fluctuations: the overall shape of the xenon agglomerate is still mostly present, but large density blobs arise along the filament line. The lowest brightness that still carries some structural information is reported in Fig. S8f. There, the fluctuations in the density values of xenon are so strong that some parts of the structure are missing. The correspondence with the original structure is barely perceivable, but still present.

Finally, at a photon count of  $1.0 \cdot 10^6$ , most of the structural information is completely lost, with little or no direct connection between the original filament shapes and the retrieved densities, which show noisy artifacts

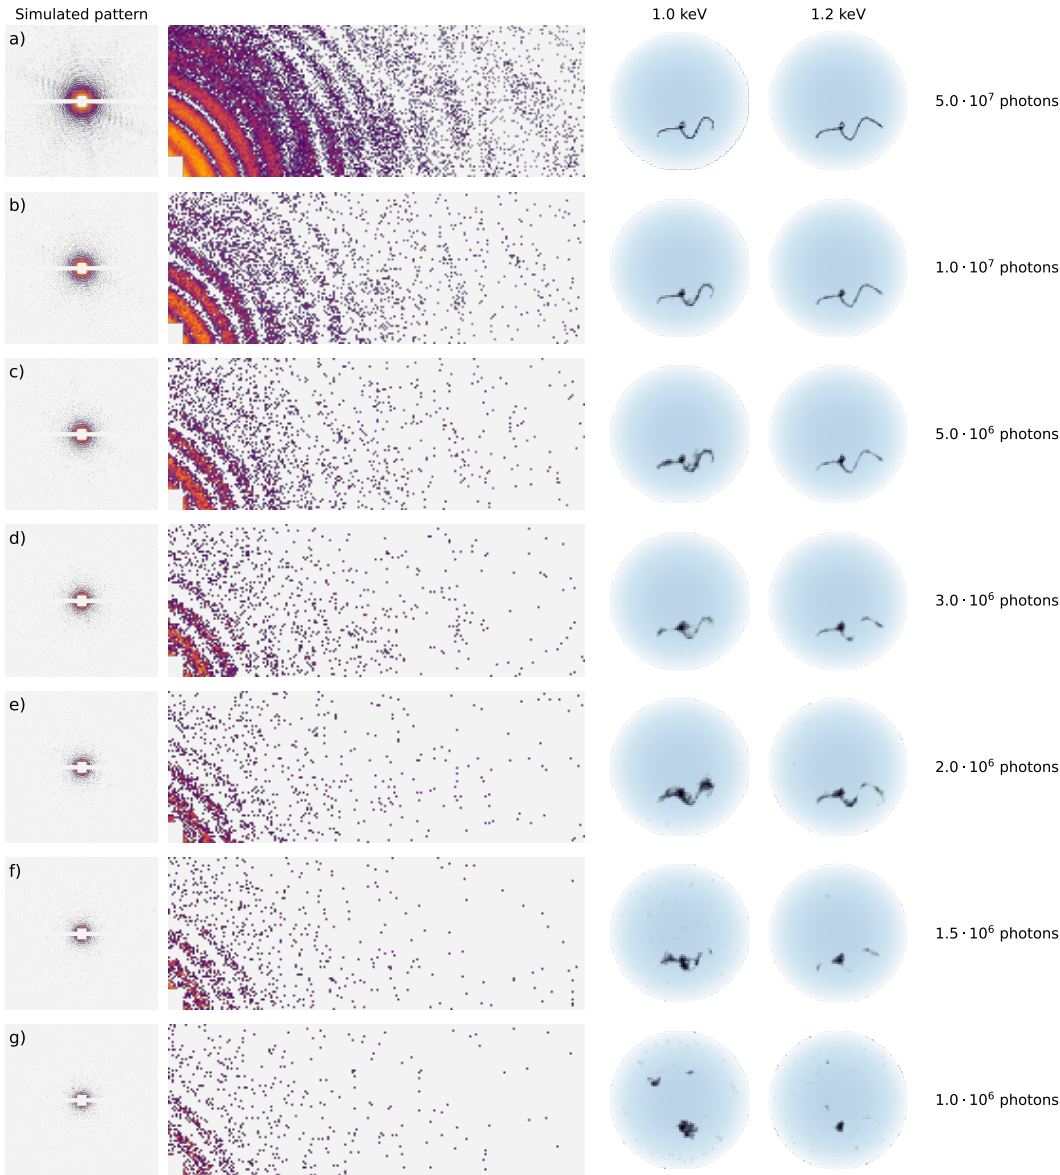

Figure S8: Impact of different brightness on the *Dichography* performance when combined with the DCDI method. Each row, from a) to g), deals with a scattering simulation of the same system, for different intensities of the recorded scattering signals. The first column corresponds to the simulated diffraction data, with a zoomed-in region reported in the second column, to better visualize the photon statistics. The third and fourth columns report the two frames of the *Dichography* reconstruction, for the 1.0 keV and the 1.2 keV, respectively. At the end of each row, the total number of scattered photons is indicated.

distributed all around the droplet, with no structural correspondence even between the two frames.

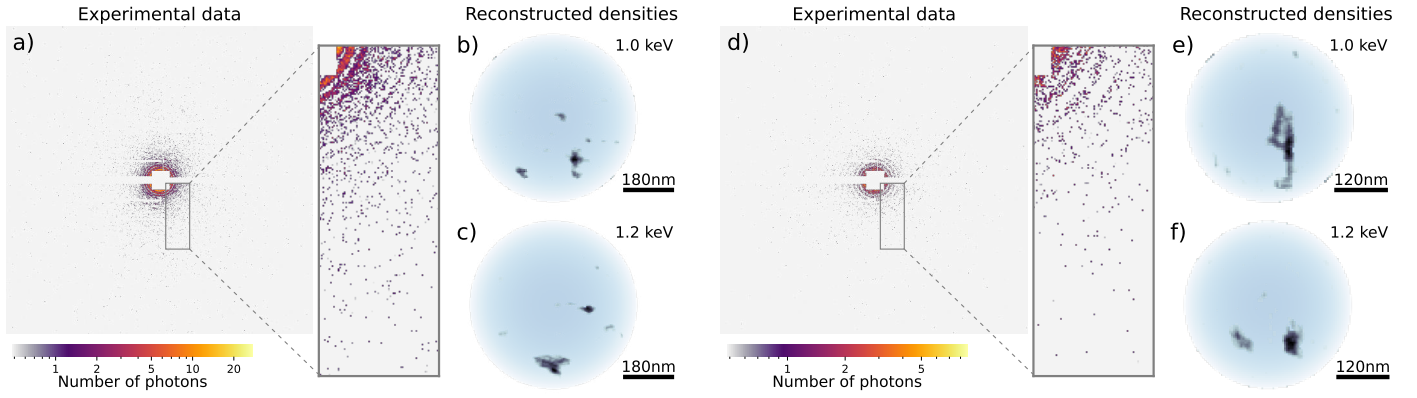

Figure S9: Examples of failed reconstructions from two-color diffraction patterns. The experimental diffraction patterns are reported in a) and d), on which the diffraction signals produced by two different photon energies, 1.0 keV and 1.2 keV, overlap. The intensity is encoded as reported by the color bar at the bottom. The intensity values are translated into numbers of 1.2 keV photons per pixel. The inset plot is a zoomed-in region of the diffraction image, to better appreciate the photon statistics, and thus the statistical noise, that affects the experimental data. The two reconstructed frames of the electronic density are reported in b), c) and e), f) for the patterns in a) and d), respectively. In particular, b) and e) report the reconstruction from the 1.0 keV pulse, while c) and f) correspond to the 1.2 keV pulse.

### S1.5 Examples of failed two-color reconstructions

In this section we show additional reconstructions of two-color data, where imaging failed, i.e., where the structures reconstructed in the two frames, corresponding to the two views on the sample by different colors, are inconsistent. Examples of failed reconstructions are shown in Fig. S9. It is worth noting that the features of the reconstructed frames, in Fig. S9b and Fig. S9c for the pattern in Fig. S9a, and in Fig. S9e and Fig. S9f for the pattern in Fig. S9d, closely resemble what observed in the simulated data for the low photon yield in Fig. S8g. Fig. S9 aims at giving a more consistent view on the reconstruction quality, and at making the reader more aware of the significance of the results presented in Fig. 4 of the main manuscript, despite their low signal-to-noise ratio and the presence of artifacts.

## S2 Spatial separation for double-hit patterns

When two particles are simultaneously present in the interaction region, they both scatter their own field. The two fields interact, introducing an interference term in the recorded data. However, the frequency of the interference term is proportional to the spatial separation between the particles: the larger the distance, the higher the oscillation frequency of the interference. When the signal oscillation of the interference is smaller than the sampling capabilities of the detector, this part of the signal is lost. In this case, the data can be employed for *Dichography*, as discussed in Appendix D 1 of the main manuscript in the case of silver nanoparticles investigated at SwissFEL.

Here, we simulate the diffraction signal for different distances between the nanoparticles in the direction transverse to the FEL propagation axis, and we show under which conditions the interference term is captured, or not, by the detector. A first example is given in Fig. S10, for a  $2048 \times 2048$  pixel detector. This simulation is similar to the actual experimental conditions, where the 4 megapixel Jungfrau detector is employed [4]. To match the experiment, also the photon energy is adjusted to 1 keV and the maximum acquired scattering angle is set to  $13.5^\circ$ . Fig. S10 shows, in addition to the diffraction pattern for the different distances and a zoomed region to better highlight the interference signal, also the autocorrelation function of the sample. This can be obtained via a direct Fourier Transform (FT) of the simulated scattering.

The autocorrelation function is a precious indicator, as it makes straightforward to recognize if the interference term is contained, or not, in the recorded data. In particular, the central peak of the autocorrelation is the convolution of the individual particles with themselves. The two additional peaks come, instead, from the cross-correlation between one particle and the other, and it can only appear if the interference between the two particles is correctly sampled. Fig. S10 shows that, employing the full-resolution data, interference is resolved up to  $3.5 \mu\text{m}$ .

Fig. S11 and Fig. S12 are the same simulations performed instead for detectors with  $1024 \times 1024$  and  $512 \times 512$  pixel dimensions, with the other experimental parameters unchanged. A reduction of the sampling capabilities impacts the maximum distance at which interference is resolved. For example, for a  $1024 \times 1024$  pixel detector, interference is already lost at a distance of  $2 \mu\text{m}$ . This distance reduces to less than  $1 \mu\text{m}$  for a  $512 \times 512$  pixel count.

All double-hit reconstructions of silver nanoparticles used a diffraction pattern rescaled to  $512 \times 512$  via a binning operation, artificially reducing the sampling capability of the detector. So, in this case, a separation of  $1 \mu\text{m}$  between the particles suffices to avoid the interference term and to make the data compatible with *Dichography*.

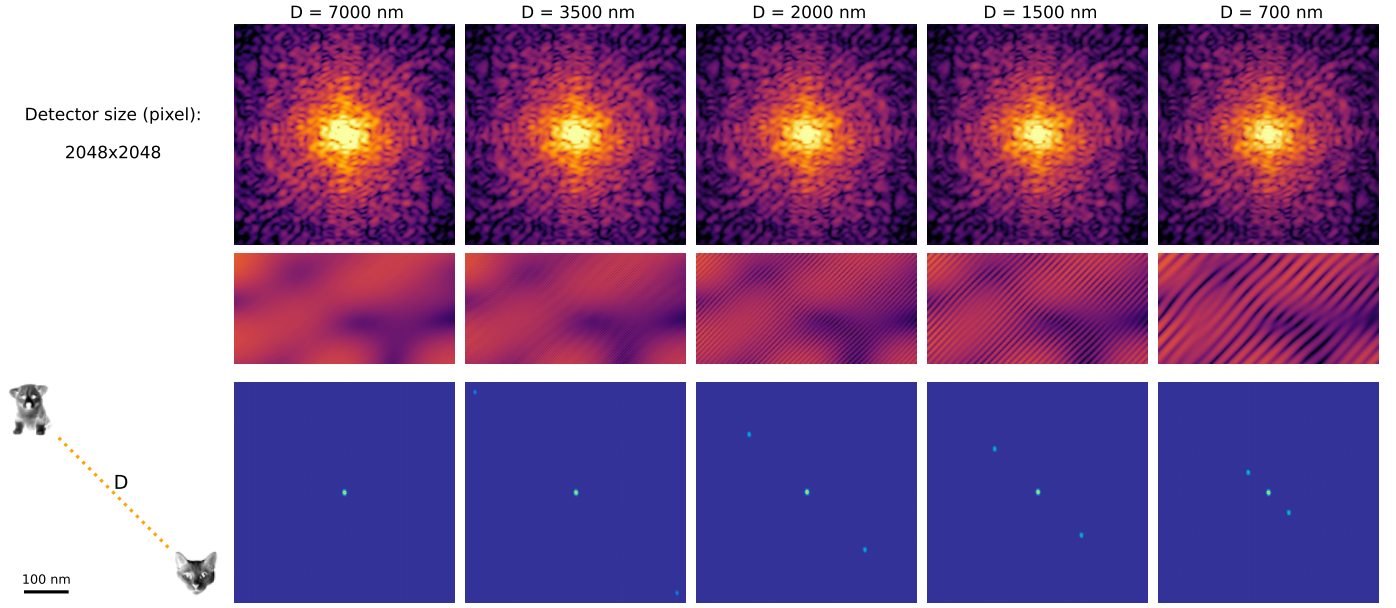

Figure S10: Simulation of a double-hit pattern as a function of the particle distance  $D$  for a  $2048 \times 2048$ -pixel detector, with geometry and photon energy equivalent to those of the SwissFEL experiment. Each column corresponds to a different distance between the two particles. The first row shows the simulated diffraction pattern. The second row displays a cropped region of the pattern to make the interference signal more visible. The last row shows the autocorrelation function of the system, obtained by an inverse Fourier transform of the pattern.

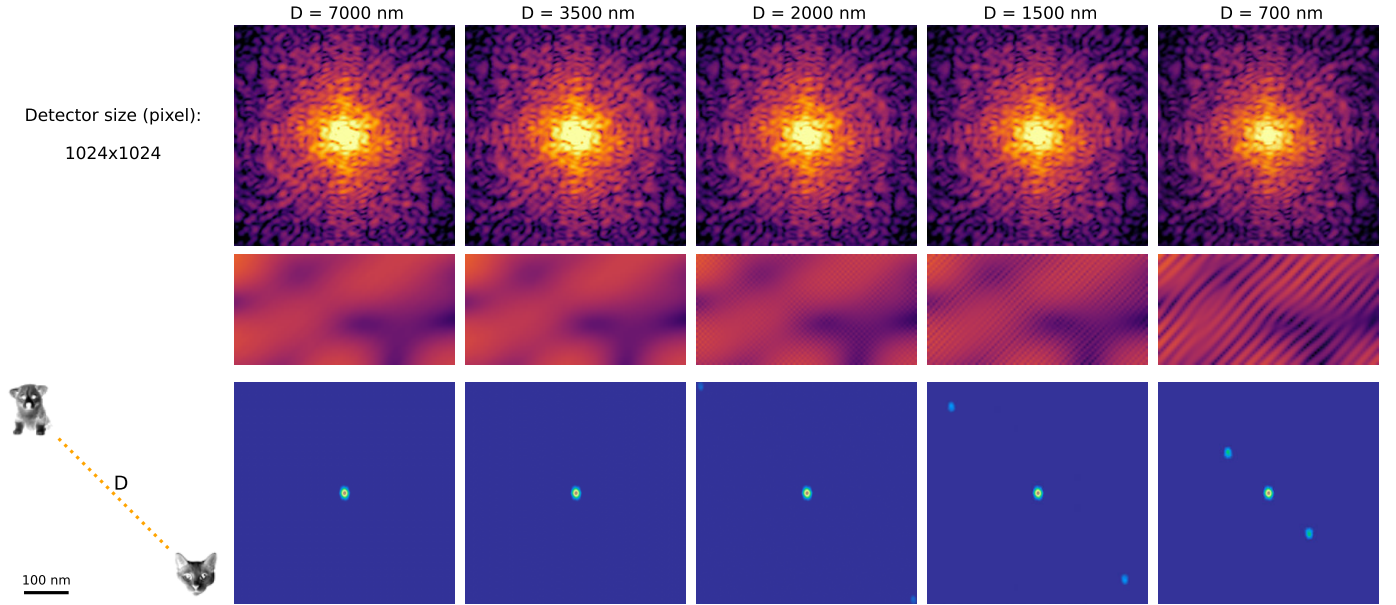

Figure S11: Simulation of a double-hit pattern as a function of the particle distance  $D$  for a  $1024 \times 1024$ -pixel detector, with geometry and photon energy equivalent to those of the SwissFEL experiment. Each column corresponds to a different distance between the two particles. The first row shows the simulated diffraction pattern. The second row displays a cropped region of the pattern to make the interference signal more visible. The last row shows the autocorrelation function of the system, obtained by an inverse Fourier transform of the pattern.

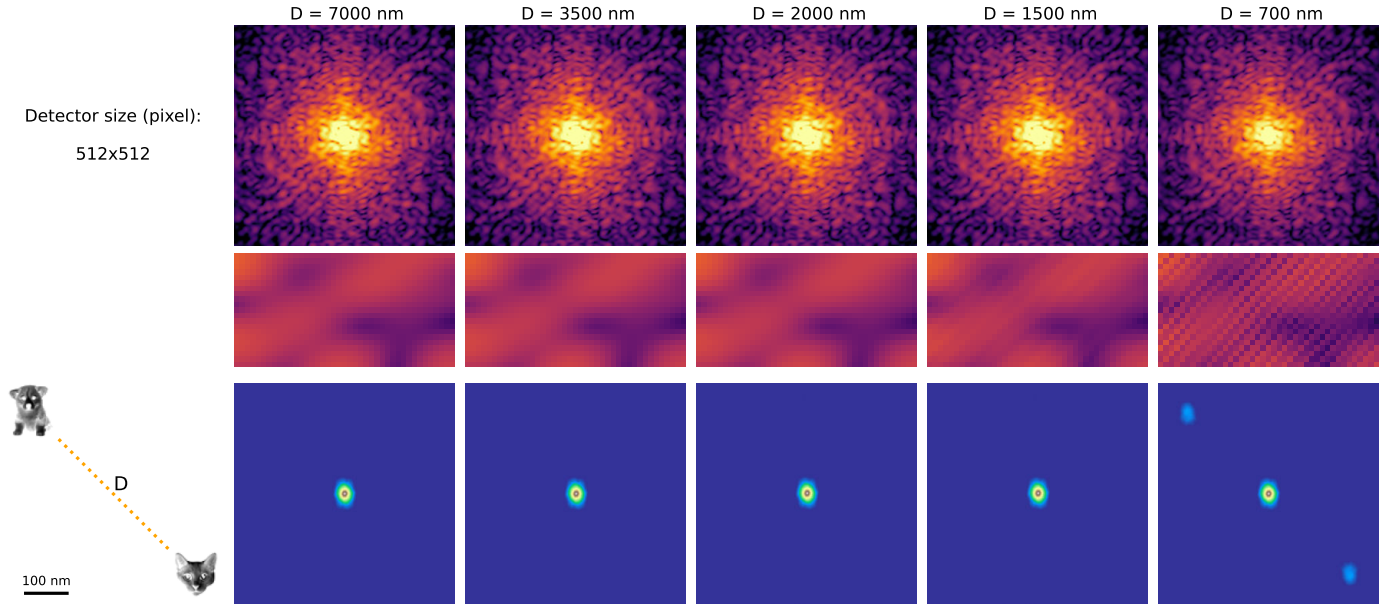

Figure S12: Simulation of a double-hit pattern as a function of the particle distance  $D$  for a  $512 \times 512$ -pixel detector, with geometry and photon energy equivalent to those of the SwissFEL experiment. Each column corresponds to a different distance between the two particles. The first row shows the simulated diffraction pattern. The second row displays a cropped region of the pattern to make the interference signal more visible. The last row shows the autocorrelation function of the system, obtained by an inverse Fourier transform of the pattern.

### S3 The intensity constraint

*Dichography* employs an adapted version of the *intensity projector* of conventional CDI [5], as introduced in Appendix A 2 of the main text. Here we present a more formal definition of the mathematical operations that are used to *back-propagate* the experimental information to the two frames of the reconstruction.

Given  $\psi_{ij}^A$  and  $\psi_{ij}^B$  the matrices containing the current field estimates of  $\rho^A$  and  $\rho^B$ , obtained with a Fourier Transform (FT) operation, we define the tensor  $\mathcal{V} \in \mathbb{C}^2$ . Its entries at coordinates  $i, j$  are defined as:

$$\mathcal{V}_{ij} = \begin{pmatrix} \psi_{ij}^A \\ \psi_{ij}^B \end{pmatrix} \quad (\text{S7})$$

In simple terms, the tensor  $\mathcal{V}$  is formed by stacking the two fields  $\psi_{ij}^A$  and  $\psi_{ij}^B$ . Eq. (S7) allows us to express the condition in Eq. (A1) of the main text in the following, formal but compact, form:

$$\|\mathcal{V}_{ij}\| = \sqrt{I_{ij}} \quad (\text{S8})$$

where  $\|\cdot\|$  indicates the  $L^2$  norm.

The enforcing of the Fourier intensity constraint can be thus reduced to a trivial renormalization of the entries in the matrix  $\mathcal{V}_{ij}$ . Given  $\mathcal{V}$  containing the current field estimates  $\psi^A$  and  $\psi^B$ , a new tensor  $\mathcal{V}'$  can be created as:

$$\begin{aligned} \mathcal{V}'_{ij} &= \frac{\mathcal{V}_{ij}}{\|\mathcal{V}_{ij}\|} \cdot \sqrt{I_{ij}} \\ &= \begin{pmatrix} \frac{\psi_{ij}^A}{\sqrt{|\psi_{ij}^A|^2 + |\psi_{ij}^B|^2}} \cdot \sqrt{I_{ij}} \\ \frac{\psi_{ij}^B}{\sqrt{|\psi_{ij}^A|^2 + |\psi_{ij}^B|^2}} \cdot \sqrt{I_{ij}} \end{pmatrix} \\ &= \begin{pmatrix} \psi_{ij}^{A'} \\ \psi_{ij}^{B'} \end{pmatrix}. \end{aligned} \quad (\text{S9})$$

It is straightforward to verify that, for each  $i, j$ ,  $\mathcal{V}'_{ij}$  satisfies the condition in Eq. (S8), i.e. its components  $\psi_{ij}^{A'}$  and  $\psi_{ij}^{B'}$  fulfill Eq. (A1). In simple terms, the magnitude of each of the two fields  $\psi_{ij}$  is corrected by a factor  $\frac{\sqrt{I_{ij}}}{\sqrt{|\psi_{ij}^A|^2 + |\psi_{ij}^B|^2}}$ . It is, furthermore, trivial to verify that the operation in Eq. (S9) is a *projection* operation, thus retaining the mathematical properties of its counterpart in conventional CDI [5].

### S4 Behavior of the iterative algorithms

The modified *intensity constraint* described in Appendix A 2 of the main text allows for a straightforward adaptation of the conventional iterative phase retrieval (IPR) algorithms [5] to *Dichography*. As reported in Appendix A 1, the reconstruction of the two frames is built upon two separate IPR procedures, which are entangled via the intensity constraint in Fourier space while remaining independent in real space through the application of the *support constraint*.

Among the different IPR algorithms that can be implemented, the Error Reduction algorithm (ER) is of particular importance for conventional CDI. It takes its name from the fact that it is a *steepest-descent* method for the error function, i.e., the error value is always reduced at each iteration [6]. The *Dichography* intensity constraint retains the original property of being a *projection* operation [5]. However, the link between the real space, where the support function is constrained, and the reciprocal space, where the experimental intensities

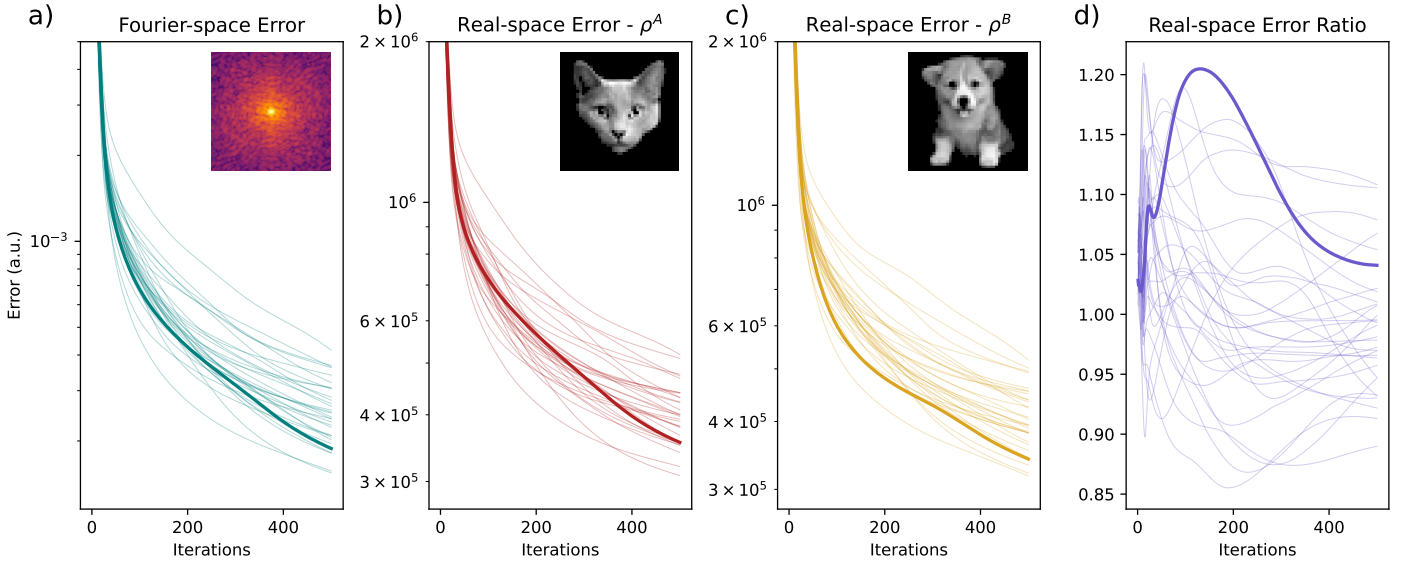

Figure S13: Typical behavior of the error value for the *dichographic* version of the Error Reduction algorithm is reported for 32 different reconstruction attempts of 500 iterations each. The error value computed in Fourier space is plotted in a). Instead, b) and c) report the error value calculated in real space, which is separated for the two frames. The ratio between the real-space errors of  $\rho^A$  and  $\rho^B$  is plotted in d), to underline how the two frames can differently contribute to the overall error value. The thick line in each plot highlights the behavior of a single, randomly selected, reconstruction process.

are constrained, is no longer a plain Fourier transform. One implication is that the norm is not preserved and, thus, the ER algorithm loses its strictly *steepest-descent* characteristics in the *dichographic* version.

In this section, we investigate the behavior of the error with proceeding algorithm iterations and highlight some peculiarities of the iterative phase retrieval algorithms adapted to *Dichography*.

The error value is evaluated as the difference between the recorded diffraction pattern and the current estimate of the field. For *Dichography*, the error of a reconstruction for two given frames  $\rho^A$  and  $\rho^B$  can be evaluated as:

$$\mathcal{E}[\rho^A, \rho^B] = \left\| \sqrt{|\mathcal{F}[\rho^A \cdot S^A]|^2 + |\mathcal{F}[\rho^B \cdot S^B]|^2} - \sqrt{I} \right\| \quad (\text{S10})$$

where  $S^A, S^B$  are the support functions of the two frames, and the operations  $\rho \cdot S$  set to zero the density values outside the support function. The operation in Eq. (S10) calculates in Fourier space the Euclidean distance ( $L^2$  norm) between the current estimate and the experimentally measured scattering amplitude. The typical error behavior with ER iterations observed in *Dichography* is reported in Fig. S13a. An interesting feature of the reported error value is that it is systematically reduced over iterations, i.e., the algorithm behaves here as a *steepest-descent* method, despite this not being mathematically ensured.

A further error value can be calculated in real space by computing the  $L^2$  norm of those coordinates outside the support constraint. For conventional CDI, the two ways of calculating the error are equivalent because of the *Parseval theorem*, as the FT operation preserves the  $L^2$  norm. For *Dichography*, the link between the two spaces is more than a plain FT, and this strict link no longer holds.

In fact, in this case the error in real space can provide more insight, as the contributions to the error value from the two frames  $\rho^A$  and  $\rho^B$  can be independently computed. The behavior of the *real-space* error is reported in Fig. S13b and Fig. S13c for  $\rho^A$  and  $\rho^B$ , respectively. One of the 32 error traces, coming from 32 independent reconstructions, is highlighted to show the typical overall behavior. The real-space errors in Fig. S13b and Fig. S13c reveal that the error for both frames is decreasing, but their behaviors — and thus their contributions to the total error (Fig. S13a) — can differ and change during the process. This aspect is better illustrated in

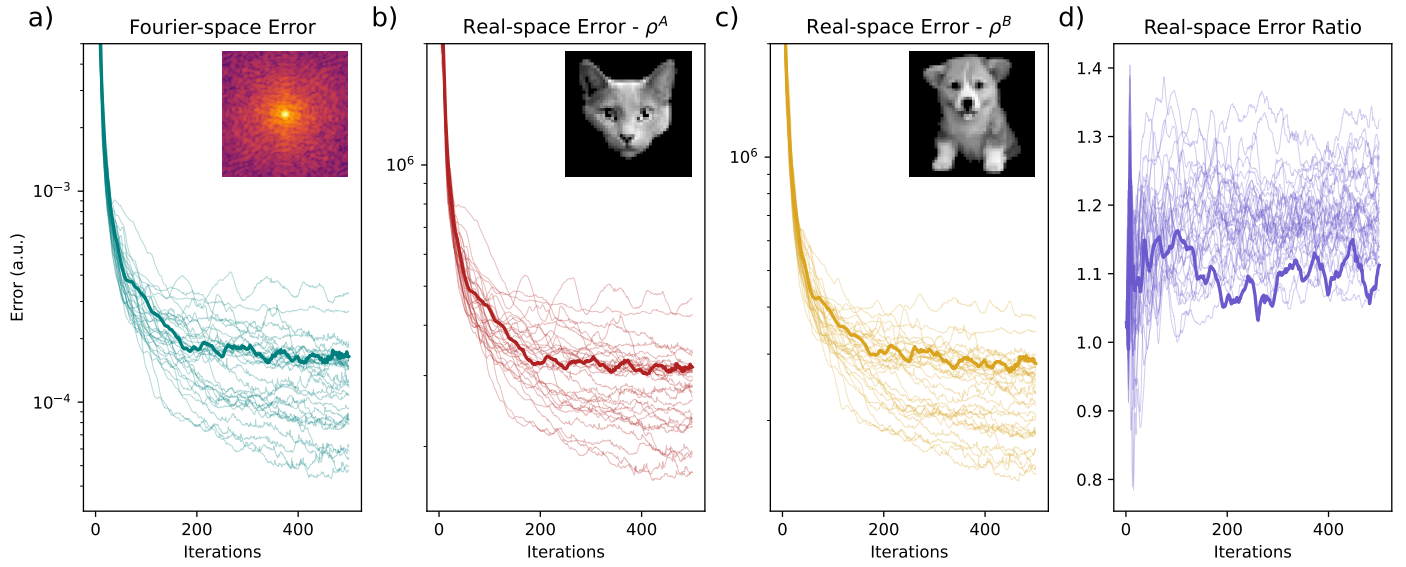

Figure S14: Typical behavior of the error value for the *dichographic* version of the Hybrid Input-Output algorithm, reported for 32 different reconstruction attempts of 500 iterations each. The error value computed in Fourier space is plotted in a). Instead, b) and c) report the error value calculated in real space, which is separated for the two frames. The ratio between the real-space errors of  $\rho^A$  and  $\rho^B$  is plotted in d), to underline how the two frames can differently contribute to the overall error value. The thick line in each plot highlights the behavior of a single, randomly selected, reconstruction process.

Fig. S13d, where the ratio between the two real-space errors of  $\rho^A$  and  $\rho^B$  is reported. Fluctuations of the ratio away from 1 indicate an imbalance in the error contributions.

A similar investigation of the error behavior can be accomplished in the case of the *dichographic* adaptation of the Hybrid Input-Output (HIO) algorithm [6], and is reported in Fig. S14. The HIO behavior retains the properties observed in conventional CDI, with a higher capability of reducing the error value when the reconstruction is far from the solution. In fact, the error reached by ER in Fig. S13 is significantly higher than the one reached by HIO after the same number of iterations.

The well-known drawback of the HIO algorithm is, however, its instability, visible in the strong fluctuations of the error value in Fig. S14. The usual approach in conventional CDI is to start a reconstruction attempt with the HIO algorithm, and then use the ER algorithm to improve the convergence properties. The same approach is undertaken in the error analysis shown in Fig. S15, where the first 200 iterations are performed with the HIO algorithm, and the following ones with the ER algorithm.

A first consideration regards the overall error value reached after 500 iterations, which is lower than both the ER-only attempt (Fig. S13) and the HIO-only attempt (Fig. S14), confirming that alternating the two algorithms is a more convenient approach, similar to what has been observed for conventional CDI.

A second note concerns the zoomed-in region reported in Fig. S15a, where a localized increase in the error value is observed despite the use of the ER algorithm. This behavior confirms that the ER algorithm loses its *steepest-descent* feature, as the error value can actually increase with subsequent iterations. However, we empirically observe that the increase in the error during ER iterations only occurs locally, and in practice the algorithm appears to retain its *steepest-descent* properties over the scale of several iterations.

A deeper mathematical investigation of *Dichography* and a more formal treatment of the problem is strongly encouraged by the authors, as it may lead to the development of better and more efficient algorithmic operations, as well as a more suitable definition of the error value of a reconstruction.

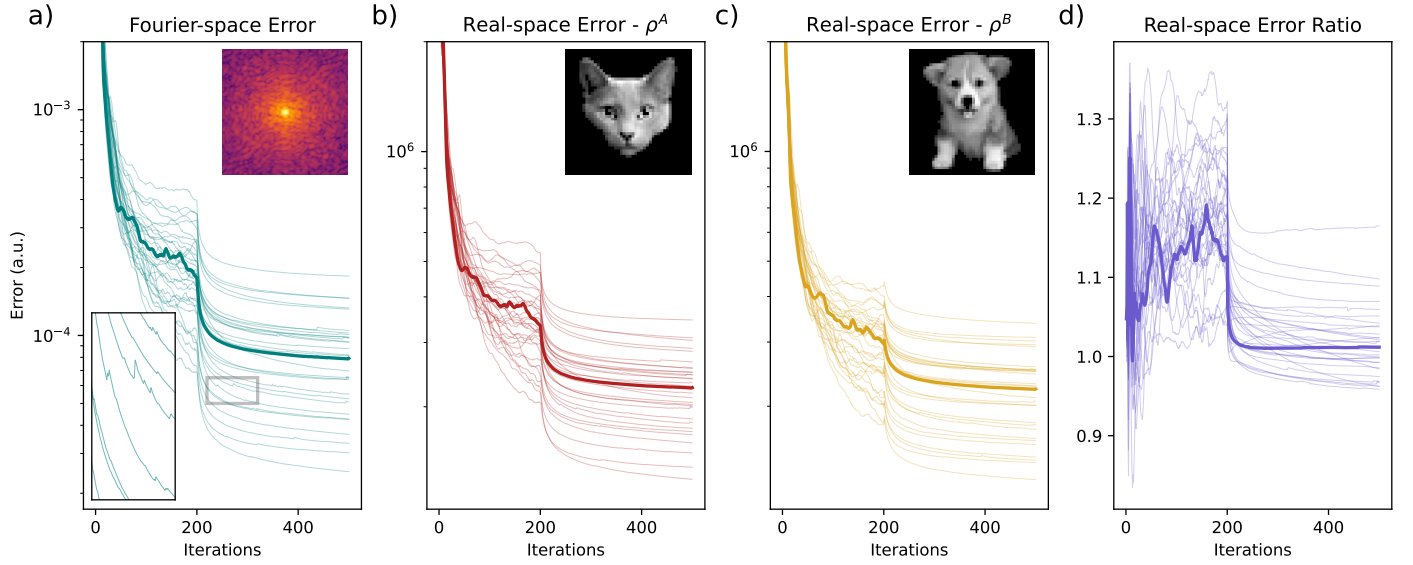

Figure S15: Typical behavior of the error value for a combination of 200 iterations of HIO followed by 300 iterations of ER algorithm, reported for 32 different reconstruction attempts. The error value computed in Fourier space is plotted in a), wherein the inset plot is a zoom-in of the region highlighted by the gray rectangle. Instead, b) and c) report the error value calculated in real space, which is separated for the two frames. The ratio between the real-space errors of  $\rho^A$  and  $\rho^B$  is plotted in d), to underline how the two frames can differently contribute to the overall error value. The thick line in each plot highlights the behavior of a single, randomly selected, reconstruction process.

## S5 Maximum number of ejected photoelectrons from a helium nanodroplet

When a helium nanodroplet is irradiated with X-ray pulses, the electrons in the system can be ejected via the photoelectric effect. The maximum number of photoelectrons  $n_{e,\text{out}}$  that can leave the droplet depends on the balance between the photon energy and the Coulomb potential generated by the accumulated positive charge on the droplet. This maximum number can be estimated by equating the excess photon energy (above the ionization potential  $I_p$ ) to the Coulomb potential created by the droplet charge [7]:

$$n_{e,\text{out}} = \frac{(E_{\text{ph}} - I_p) 4\pi\epsilon_0 R}{e^2}, \quad (\text{S11})$$

where  $R$  is the droplet radius,  $E_{\text{ph}}$  is the photon energy,  $I_p$  is the ionization potential and  $e$  is the elementary charge. For a helium ( $I_p = 24.6 \text{ eV}$ ) nanodroplet of size  $R = 350 \text{ nm}$  illuminated by  $1 \text{ keV}$  radiation, Eq. (S11) gives a maximum number of photoelectrons of  $n_{e,\text{out}} = 2.4 \cdot 10^5$  emitted, before the Coulomb potential prevents further electron escape.

### S5.1 Expected dynamics of ejected ions

The maximum number of ejected photoelectrons corresponds to the maximum charge accumulated in the system. Charged ions are subjected to a Coulomb repulsion and accelerated outwards. The kinetic energy  $E_{\text{kin}}(r)$  of an ion at a distance  $r > R$  from the center of the droplet can be calculated as:

$$E_{\text{kin}}(r) = \frac{qQ}{4\pi\epsilon_0} \left( \frac{1}{R} - \frac{1}{r} \right). \quad (\text{S12})$$

The corresponding velocity is:

$$v(r) = \sqrt{\frac{2E_{\text{kin}}(r)}{m}} = \sqrt{\frac{qQ}{2m\pi\epsilon_0} \left( \frac{1}{R} - \frac{1}{r} \right)}, \quad (\text{S13})$$

where  $m$  is the mass of the helium ion.

Expressing velocity as  $v = \frac{dr}{dt}$ , we can write:

$$\frac{dr}{dt} = \sqrt{\frac{qQ}{2m\pi\epsilon_0} \left( \frac{1}{R} - \frac{1}{r} \right)}. \quad (\text{S14})$$

Rearranging and integrating from the droplet surface  $r = R$  at  $t = 0$  to  $r = R + \Delta r$  at time  $t$ :

$$t = \sqrt{\frac{2m\pi\epsilon_0}{qQ}} \int_R^{R+\Delta r} \frac{dr'}{\sqrt{\frac{1}{R} - \frac{1}{r'}}}. \quad (\text{S15})$$

This expression gives the time required for a singly charged helium ion to move a distance  $\Delta r$  away from the droplet surface under Coulomb repulsion. The following values are numerically calculated from Eq. (S15):

| Time [fs] | Distance [nm] |
|-----------|---------------|
| 50        | 0.09          |
| 750       | 18.75         |
| 1500      | 70.85         |

## Supplementary References

- [1] R. M. P. Tanyag, C. Bernando, C. F. Jones, C. Bacellar, K. R. Ferguson, D. Anielski, R. Boll, S. Carron, J. P. Cryan, L. Englert, *et al.*, “Communication: X-ray coherent diffractive imaging by immersion in nanodroplets,” *Structural Dynamics*, vol. 2, no. 5, 2015.
- [2] A. Ulmer, A. Heilrath, B. Senfftleben, S. M. O’Connell-Lopez, B. Kruse, L. Seiffert, K. Kolatzki, B. Langbehn, A. Hoffmann, T. M. Baumann, *et al.*, “Generation of large vortex-free superfluid helium nanodroplets,” *Physical review letters*, vol. 131, no. 7, p. 076002, 2023.
- [3] R. M. P. Tanyag, C. F. Jones, C. Bernando, S. M. O. O’Connell, D. Verma, and A. F. Vilesov, “CHAPTER 8. Experiments with Large Superfluid Helium Nanodroplets,” in *Theoretical and Computational Chemistry Series* (O. Dulieu and A. Osterwalder, eds.), pp. 389–443, Cambridge: Royal Society of Chemistry, 2017.
- [4] A. Mozzanica, M. Andrä, R. Barten, A. Bergamaschi, S. Chirioti, M. Brückner, R. Dinapoli, E. Fröjdh, D. Greiffenberg, F. Leonarski, *et al.*, “The jungfrau detector for applications at synchrotron light sources and xfels,” *Synchrotron Radiation News*, vol. 31, no. 6, pp. 16–20, 2018.
- [5] S. Marchesini, “Invited article: A unified evaluation of iterative projection algorithms for phase retrieval,” *Rev. Sci. Instrum.*, vol. 78, no. 1, p. 011301, 2007.
- [6] J. R. Fienup, “Phase retrieval algorithms: a comparison,” *Appl. Opt.*, vol. 21, no. 15, pp. 2758–2769, 1982.
- [7] C. Bostedt, H. Thomas, M. Hoener, T. Möller, U. Saalman, I. Georgescu, C. Gnodtke, and J.-M. Rost, “Fast electrons from multi-electron dynamics in xenon clusters induced by inner-shell ionization,” *New J. Phys.*, vol. 12, p. 083004, Aug. 2010.
